# Supplementary material for: On the Bottleneck of Graph Neural Networks and its Practical Implications
Source: arXiv:2006.05205 source file (2021-03-09)
Supplement: Supplementary file 1 [file combinatorial-additional.tex]

\section{Combinatorial Analysis}
\label{sec:stats-additional}
We analyize the  combinatorial upper bound for the maximal depth that a GNN can perfectly fit (learn to 100\% training accuracy) given its hidden vector size $d$. 
We denote the arity of such a tree by $m$ ($=$$2$ in our experiments);
the counting base as $b$$=$$2$; %
the number of bits in a floating-point variable as $f$$=$$32$; %
and the hidden dimension of the GNN, i.e., the size of a node vector 
$\mathbf{h}_v^{\left(k\right)}$, as $d$.

A full tree of arity $m$ has $m^{depth}$ leaves.
As described in \Cref{subsec:synthetic}, given an arrangement of blue neighbors, all possible permutations of the labels \{A, B, C, ...\} are valid. Thus, the number of leaf label assignments is $\left(m^{depth}\right)!$.
Right before interacting with the target node and predicting the label, a single vector of size $d$ must encapsulate the information flowing from all leaves (\Cref{eq:gcn,eq:gin}).\footnote{The analysis holds for GCN and GIN. Architectures that use the representation of the recipient node to aggregate messages, like GAT, need to compress the information from only \emph{half} of the leaves in a single vector. This increases the final upper bounds of $depth$ by up to 1 and demonstrated empirically in \Cref{subsec:synthetic}.}
Such a vector contains $d$ floating-point elements, each of them is stored as $f$ bits. Overall, the number of possible cases that this vector can distinguish between is $b^{f\cdot d}$. The number of possible cases that the vector can distinguish between must be greater than the number of different examples this vector may encounter in the training data. 

 \Cref{eq:dim-depth};
considering binary trees ($m$$=$$2$), and floating-point values of $f$$=$$32$ binary ($b$$=$$2$) bits, we get \Cref{eq:dim-depth-concrete}:
\newline
\noindent\begin{minipage}[t]{.5\linewidth}
\begin{equation}
	\left(m^{depth}\right)!  < b^{f\cdot d}
	\label{eq:dim-depth2}
\end{equation}
\end{minipage}
\noindent\begin{minipage}[t]{.5\linewidth}
\begin{equation}
	\left(2^{depth}\right)!  < 2^{32\cdot d}
	\label{eq:dim-depth-concrete2}
\end{equation}
\end{minipage}

Now, we can fix either $d$ or $depth$ and solve for the other. For example, in \Cref{fig:dim-depth} we fixed different values of $d$ and found the maximal $depth\in \mathbb{N}$ that satisfies \Cref{eq:dim-depth-concrete}, to get the combinatorial max $depth$ for each value of $d$.
